# Supplementary material for: Latent Bridges for Multi-Table Question Answering
Source: arXiv:2606.28916 source file (2026-10-22)
Supplement: Supplementary file 2 [file tab_stress-appendix.tex]

\begin{table*}[t]
\centering
\caption{Stress-test results. F1 and CC scores averaged over questions across 15 different tables. GRAB columns report results with the full graph encoder; serialized columns use the LLM with flattened table input only. }
\label{tab_stress_test}
\setlength{\tabcolsep}{4pt}

\small
\begin{tabular}{llcccccccc}
\toprule
& & \multicolumn{4}{c}{\textbf{Serialized only}} & \multicolumn{4}{c}{\textbf{+ GRAB}} \\
\cmidrule(lr){3-6} \cmidrule(lr){7-10}
& & \multicolumn{2}{c}{Qwen-4B} & \multicolumn{2}{c}{GPT-5.4-mini} & \multicolumn{2}{c}{Qwen-4B} & \multicolumn{2}{c}{GPT-5.4-mini} \\
\cmidrule(lr){3-4} \cmidrule(lr){5-6} \cmidrule(lr){7-8} \cmidrule(lr){9-10}
\textbf{Question type} & \textbf{Cond.} & F1 & CC & F1 & CC & F1 & CC & F1 & CC \\
\midrule
Overall \small{(2337)} & --- & 39.29 & 22.59 & 68.05 & 41.59 & 60.71 & 39.50 & --- & --- \\
\midrule
\multicolumn{10}{l}{\textit{Lookup}} \\
\quad Single condition    & AND $\times$1      & 66.59 & 37.14 & 85.55 & 64.76 & 80.72 & 58.10 & --- & --- \\
\quad Double condition    & AND $\times$2      & 65.56 & 54.29 & 93.41 & 82.86 & 89.32 & 74.29 & --- & --- \\
\quad Triple condition    & AND $\times$3      & 73.90 & 87.62 & 98.73 & 98.10 & 95.52 & 92.38 & --- & --- \\
\quad Double condition OR & OR $\times$2       & ---   & ---   & ---   & ---   & ---   & ---   & --- & --- \\
\quad Mixed condition     & OR + AND           & ---   & ---   & ---   & ---   & ---   & ---   & --- & --- \\
\midrule
\multicolumn{10}{l}{\textit{Count}} \\
\quad No condition        & ---                & 8.63  & 9.80  & 84.31 & 84.31 & 54.90 & 54.90 & --- & --- \\
\quad Single condition    & AND $\times$1      & 23.01 & 24.76 & 71.43 & 71.43 & 54.29 & 54.29 & --- & --- \\
\quad Double condition    & AND $\times$2      & 34.69 & 40.00 & 57.14 & 57.14 & 57.14 & 57.14 & --- & --- \\
\midrule
\multicolumn{10}{l}{\textit{Max}} \\
\quad No condition        & ---                & 57.67 & 62.96 & 97.53 & 97.53 & 93.83 & 93.83 & --- & --- \\
\quad Single condition    & AND $\times$1      & 52.21 & 56.19 & 97.62 & 98.10 & 85.71 & 85.71 & --- & --- \\
\quad Double condition    & AND $\times$2      & 68.76 & 75.24 & 94.76 & 95.24 & 79.05 & 79.05 & --- & --- \\
\midrule
\multicolumn{10}{l}{\textit{Avg}} \\
\quad No condition        & ---                & 1.23  & 1.23  & 1.23  & 1.23  & 1.23  & 1.23  & --- & --- \\
\quad Single condition    & AND $\times$1      & 9.38  & 14.29 & 17.14 & 17.14 & 15.24 & 15.24 & --- & --- \\
\quad Double condition    & AND $\times$2      & 28.62 & 34.29 & 46.67 & 46.67 & 40.95 & 40.95 & --- & --- \\
\midrule
\multicolumn{10}{l}{\textit{Group-by Max}} \\
\quad Single key          & G1                 & 42.92 & 4.76  & 75.60 & 35.24 & 72.59 & 48.57 & --- & --- \\
\quad Single key + filter & G1, AND $\times$1  & 43.69 & 6.67  & 59.13 & 6.67  & 70.20 & 37.14 & --- & --- \\
\quad Double key          & G2                 & 38.28 & 0.00  & 49.95 & 3.81  & 60.00 & 17.14 & --- & --- \\
\quad Double key + filter & G2, AND $\times$1  & 38.58 & 0.00  & 61.86 & 4.76  & 55.88 & 12.38 & --- & --- \\
\midrule
\multicolumn{10}{l}{\textit{Group-by Count}} \\
\quad Single key          & G1                 & 34.58 & 2.08  & 77.50 & 36.46 & 62.40 & 30.21 & --- & --- \\
\quad Single key + filter & G1, AND $\times$1  & 39.35 & 1.90  & 79.79 & 40.00 & 62.46 & 25.71 & --- & --- \\
\quad Double key          & G2                 & 37.44 & 0.00  & 62.43 & 14.58 & 62.57 & 11.46 & --- & --- \\
\quad Double key + filter & G2, AND $\times$1  & 39.70 & 0.00  & 73.74 & 19.05 & 49.84 & 7.14  & --- & --- \\
\midrule
\multicolumn{10}{l}{\textit{Group-by Avg}} \\
\quad Single key          & G1                 & 21.63 & 1.90  & 58.71 & 4.76  & 38.77 & 6.67  & --- & --- \\
\quad Single key + filter & G1, AND $\times$1  & 30.12 & 6.67  & 69.14 & 10.48 & 53.64 & 17.14 & --- & --- \\
\quad Double key          & G2                 & 27.44 & 0.00  & 50.33 & 0.95  & 49.02 & 1.90  & --- & --- \\
\quad Double key + filter & G2, AND $\times$1  & 38.46 & 0.95  & 73.14 & 16.19 & 56.59 & 14.29 & --- & --- \\
\bottomrule
\end{tabular}
\end{table*}
